# Supplementary material for: Predicting protein inter-residue contacts using composite likelihood maximization and deep learning
Source: arXiv:1809.00083 ancillary file (2018-08-31)
Supplement: Supplementary file 1 [file clmDCA_Supplementary.pdf]

# Predicting protein residue-residue contacts using composite likelihood maximization and deep learning

Haicang Zhang<sup>a,b</sup>, Qi Zhang<sup>a,b</sup>, Fusong Ju<sup>a,b</sup>, Jianwei Zhu<sup>a,b</sup>, Shiwei Sun<sup>a,b</sup>, Yujuan Gao<sup>c</sup>, Ziwei Xie<sup>e</sup>, Minghua Deng<sup>c</sup>, Shiwei Sun<sup>\*,a,1</sup>, Wei-Mou Zheng<sup>\*,d</sup>, Dongbo Bu<sup>\*,a,b</sup>

<sup>a</sup>Key lab of intelligent information processing, Institute of Computing Technology, Chinese Academy of Sciences, Beijing, China

<sup>b</sup>University of Chinese Academy of Sciences, Beijing, China

<sup>c</sup>Center for Quantitative Biology, School of Mathematical Sciences, Center for Statistical Sciences, Peking University, Beijing, China

<sup>d</sup>Institute of Theoretical Physics, Chinese Academy of Sciences, Beijing, China

<sup>e</sup>Department of Computer Science, Huazhong University of Science and Technology, Wuhan, China

---

---

## Supplementary Material

### 1. Calculation of gradients of composite likelihood

For a query protein of length  $L$ , we denote an MSA of its homologous proteins as  $\{x^m\}_{m=1}^M$ , where  $M$  denotes the number of homologous proteins, and  $x^m = (x_1^m, x_2^m, \dots, x_L^m)$  represents the  $m$ -th sequence in MSA. Each element  $x_i^m, i = 1, 2, \dots, L$ , has a total of 21 possible values, including 20 ordinary amino acid types and gap in alignment. For the sake of simplicity, we treat gap as a specific amino acid.

We use a vector of variables  $X = (X_1, X_2, \dots, X_L)$  to represent a protein sequence with  $X_i$  being the  $i$ -th residue. According to the maximum entropy principle [5], the probability that  $X$  takes the value  $x^m$  can be represented using Markov random field model [6]:

$$P(X = x^m) = \frac{1}{Z} \exp\left\{\sum_i h_i(x_i^m) + \sum_{i < j} e_{ij}(x_i^m, x_j^m)\right\} \quad (1)$$

Here the singleton term  $h_i(a)$  encodes the  $i$ -th residue's propensity for an amino acid type  $a$ , whereas the doubleton term  $e_{i,j}(a, b)$  encodes the coupling between the  $i$ -th and  $j$ -th residues when they takes amino acid types  $a$  and  $b$ , respectively.  $Z$  denotes the partition function acting as a global normalizer to ensure the probabilities sum to 1.

---

\*Correspondence should be addressed to W. Zheng (zheng@itp.ac.cn) and D. Bu (dbu@ict.ac.cn).

The optimal parameters in  $h_i$  and  $e_{i,j}$  can be solved via maximizing the likelihood (in logarithm) of all homologous proteins in MSA, i.e.,

$$\mathcal{L} = \frac{1}{M} \sum_{m=1}^M \log P(X = x^m) \quad (2)$$

The composite likelihood is defined as

$$\mathcal{CL} = \sum_{m=1}^M \sum_{c \in C} \log P(X_c = x_c^m | X_{-c} = x_{-c}^m) \quad (3)$$

Here  $C$  denotes subsets of variables, where only dependencies among variables within a subset are considered.

It should be pointed out that composite likelihood is a general model with  $\mathcal{CL}$  and  $\mathcal{PL}$  as its special cases. In particular, when setting  $C = \{\{1, 2, \dots, L\}\}$ , composite likelihood  $\mathcal{CL}$  reduces to the actual likelihood  $\mathcal{L}$ . On the contrary, when setting  $C = \{\{1\}, \{2\}, \dots, \{L\}\}$ , the composite likelihood  $\mathcal{CL}$  becomes the pseudo-likelihood  $\mathcal{PL}$ .

To match our objective of predicting residue-residue contacts, we set  $C$  as all possible residue pairs, i.e.,  $C = \{\{1, 2\}, \{1, 3\}, \dots, \{i, j\}, \dots, \{L-1, L\}\}$ . This way, the actual likelihood is approximated using pairwise composite likelihood, which explicitly represents conditional probabilities of all residue pairs as below.

$$\begin{aligned} \mathcal{CL}_{\text{pairwise}} &= \frac{1}{M} \sum_{m=1}^M \sum_{i=1}^L \sum_{j>i}^L \log P(X_{i,j} = x_{i,j}^m | X_{\neg\{i,j\}} = x_{\neg\{i,j\}}^m) \quad (4) \\ &= \frac{1}{M} \sum_{m=1}^M \sum_{i=1}^L \sum_{j>i}^L \log \frac{1}{Z_{ij}^m} \exp\{h_i(x_i^m) + h_j(x_j^m) + e_{ij}(x_i^m, x_j^m) \\ &\quad + \sum_{k \neq i, k \neq j} [e_{ik}(x_i^m, x_k^m) + e_{jk}(x_j^m, x_k^m)]\} \quad (5) \end{aligned}$$

in which

$$Z_{ij}^m = \sum_{a=1}^{21} \sum_{b=1}^{21} \exp \left\{ h_i(a) + h_j(b) + e_{ij}(a, b) + \sum_{k \neq i, k \neq j} [e_{ik}(a, X_k^m) + e_{jk}(b, X_k^m)] \right\}.$$

To find parameters  $h_i$  and  $e_{ij}$  such that  $\mathcal{CL}_{\text{pairwise}}$  is maximized, we employed the classical BFGS technique with efficient calculation of gradients.

$$\frac{\partial \mathcal{CL}_{\text{pairwise}}}{\partial h_i(a)} = (L-1)f_i(a) - \frac{1}{M} \sum_{m=1}^M \sum_{\substack{k=1 \\ k \neq i}}^L P_{i\hat{k}}^m(a) \quad (6)$$

$$\begin{aligned} \frac{\partial \mathcal{C}\mathcal{L}_{\text{pairwise}}}{\partial e_{ij}(a,b)} &= (2L-3)f_{ij}(a,b) - \frac{1}{M} \sum_{m=1}^M [P_{ij}^m(a,b) \\ &+ \sum_{\substack{k=1 \\ k \neq i, k \neq j}}^L (I(X_j^m = b)P_{ik}^m(a) + I(X_i^m = a)P_{kj}^m(b))] \end{aligned} \quad (7)$$

Table 1: Time complexity for calculating likelihood function

| Likelihood function                                    | Time complexity |
|--------------------------------------------------------|-----------------|
| Actual likelihood $\mathcal{L}$                        | NP-hard         |
| Pseudo-likelihood $\mathcal{P}\mathcal{L}$             | $O(L^2M)$       |
| Pairwise composite likelihood $\mathcal{C}\mathcal{L}$ | $O(L^2M)$       |

## 2. Pre- and post-processing, regularization, and speed-up strategies

It is very common that some homologous proteins of a query protein show considerable sequence similarity, forming redundancy in MSA. This redundancy makes the assumption of independence among homologous proteins false and the likelihood function inaccurate. To reduce the impact caused by redundancy, we pre-processed MSA by weighting all homologous proteins within it as performed by plmDCA [3] and PSICOV [4]. Similar to [2], we also applied the average-product correction (APC) technique on the predicted contacts as post-processing procedure.

The MRF model used in this study contains a total of  $O(L^2)$  parameters, usually exceeding the number of homology proteins in MSA. For example, about  $2 \times 10^7$  parameters are needed to model a query protein with length  $L = 300$ ; in contrast, few MSAs have sufficient homologous proteins for estimating these parameters, thus causing potential overfitting. To avoid overfitting, we added a penalty term to the likelihood function as follows:

$$R_{l_2} = \lambda_h \sum_{i=1}^L \|h_r\|_2^2 + \sum_{i=1}^L \sum_{j=i+1}^L \|e_{ij}\|_2^2 \quad (8)$$

To speed up likelihood maximization, we began with initial parameters calculated using plmDCA. We also exploited the parallelism in calculating gradient for residue pairs and implemented our method using OpenMP. Overall, it usually takes only a few hours for clmDCA to predict contacts for proteins with typical length of 200 amino acids.

### 3. Comparison of plmDCA and clmDCA: a case study

The two approaches, plmDCA and clmDCA, differ only in the way to calculate the parameters  $h_i$  and  $e_{ij}$  and thereafter the coupling strength  $J_{ij}$ . To reveal this difference, we examined two residue pairs, one being in contact, and the other non-contact. As shown in Figure 1 (a), the non-contact residue pair ALA183-ILE189 was incorrectly reported as being in contact by plmDCA (coupling strength:  $J_{183,189} = 1.63$ ; rank: 14th). In comparison, this pair was ranked 2053th by clmDCA (coupling strength:  $J_{183,189} = 0.05$ ) and was not reported as being in contact.

Figure 1 (b) shows THR75-MSE97 as an example of contacting residue pair. This pair was ranked 40th by plmDCA due to its considerably small coupling strength  $J_{75,97} = 1.34$ . On the contrary, clmDCA calculated the coupling strength as 0.58 (rank: 12th) and thus correctly reported it as a contact.

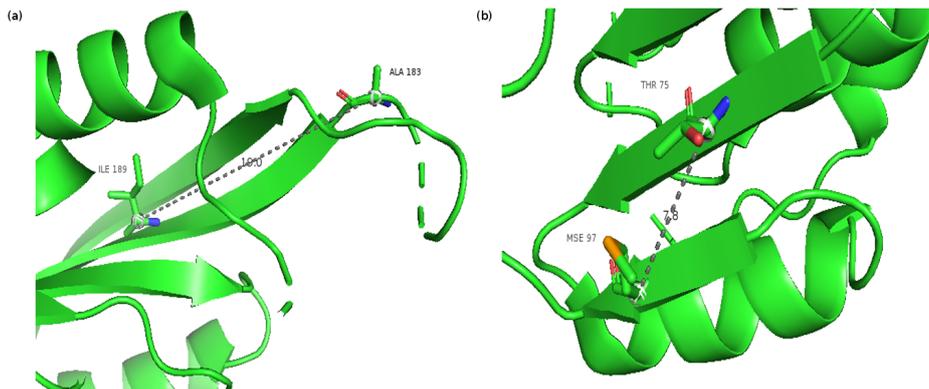

Figure 1: Two residue pairs in protein 1ne2A. (a) Non-contact residue pair ALA183-ILE189 and (b) Contacting residue pair THR75-MSE97.

### 4. Building protein 3D structures using the predicted inter-residue contacts

We further applied the predicted inter-residue contacts to build 3D structures of query proteins. For this aim, we run CONFOLD [1] with predicted contacts as input. CONFOLD builds protein structure that satisfies the input inter-residue contacts as well as possible. Previous studies have shown that knowing only a few true contacts is sufficient for building high-quality 3D structures [7].

Figure 2 compares the quality of structures built using top  $L$  contacts predicted by plmDCA, clmDCA alone, and clmDCA together with deep learning. When using contacts predicted by clmDCA alone, the quality of

built structures are the same to those built using contacts by plmDCA; however, the combination of clmDCA and deep learning technique showed substantial advantage. Specifically, when using top  $L$  contacts predicted by plmDCA as input, we successfully built high-quality structures for 77 proteins in the PSICOV dataset (TMscore  $> 0.6$ ). In contrast, we built high-quality structures for 78 proteins when using predicted contacts by clmDCA. By enhancing clmDCA with deep learning technique, the number of high-quality predictions further increased to 80.

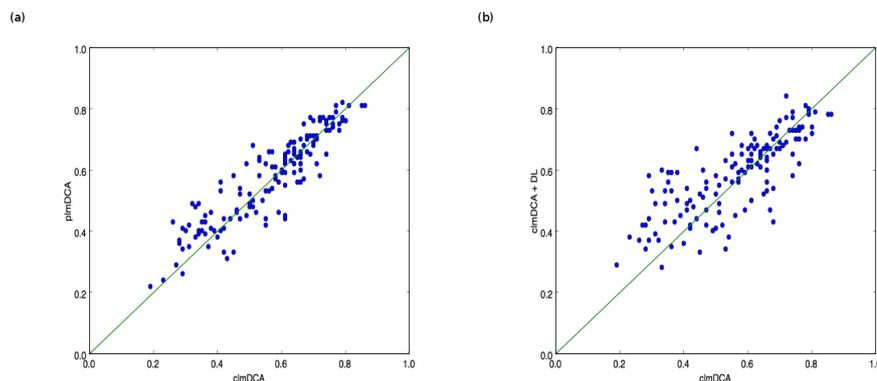

Figure 2: Comparison of quality of structures built using predicted contacts by (a) clmDCA vs. plmDCA. (b) clmDCA alone version clmDCA together with refinement using deep learning. Here protein quality is measured using TMscore. Data set: PSICOV.

- [1] Adhikari, B., Bhattacharya, D., Cao, R., and Cheng, J. (2015). CONFOLD: Residue-residue contact-guided ab initio protein folding. *Proteins*, **83**(8), 1436–1449.
- [2] Dunn, S. D., Wahl, L. M., and Gloor, G. B. (2008). Mutual information without the influence of phylogeny or entropy dramatically improves residue contact prediction. *Bioinformatics*, **24**(3), 333–340.
- [3] Ekeberg, M., Lövkvist, C., Lan, Y., Weigt, M., and Aurell, E. (2013). Improved contact prediction in proteins: using pseudolikelihoods to infer potts models. *Physical review. E, Statistical, nonlinear, and soft matter physics*, **87**(1), 12707.
- [4] Jones, D. T., Buchan, D. W., Cozzetto, D., and Pontil, M. (2012). PSICOV: precise structural contact prediction using sparse inverse covariance estimation on large multiple sequence alignments. *Bioinformatics*, **28**(2), 184–190.
- [5] Lapedes, A. S., Giraud, B., Liu, L., and Stormo, G. D. (1999). Correlated mutations in models of protein sequences: phylogenetic and structural effects. In *Statistics in molecular biology and genetics*, volume 33 of *Lecture Notes–Monograph Series*, pages 236–256.
- [6] Morcos, F., Pagnani, A., Lunt, B., Bertolino, A., Marks, D. S., Sander, C., Zecchina, R., Onuchic, J. N., Hwa, T., and Weigt, M. (2011). Direct-coupling analysis of residue coevolution captures native contacts across many protein families. *Proceedings of the National Academy of Sciences*, **108**(49), 1293–1301.
- [7] Ovchinnikov, S., Kim, D. E., Wang, R. Y.-R., Liu, Y., DiMaio, F., and Baker, D. (2016). Improved de novo structure prediction in CASP11 by incorporating coevolution information into Rosetta. *Proteins*, **84**(S1), 67–75.
